# Supplementary material for: CoT: Decentralized Elastic Caches for Cloud Environments
Source: arXiv:2006.08067 source file (2020-06-18)
Supplement: Supplementary file 1 [file appendix.tex]

\begin{appendices}

\section{Effect of Tracker Size on \algoname's Hit 
Rate}~\label{sec:tracker_size}

This experiment measures the effect of varying the tracker size while fixing
the cache size on \algoname's hit rate. The results of this experiments are
reported in Figure~\ref{fig:tracker_size}. The \textit{x-axis} is in $log_2$ 
scale and it represents the tracker size expressed as the number of tracked 
keys. The \textit{y-axis} represents the obtained cache hit rates (\%)
during a 10 million accesses experiment. In this experiment, a Zipfian access 
distribution with a skew parameter value s = 0.99 is used. Each line
in Figure~\ref{fig:tracker_size} represents the changes on the obtained 
cache hit rate when the cache size is fixed and the tracker size is varied. 
The experiment is run for different cache sizes 
(C = 1, 3, 7, 15, 31, 63, 127, 255, and 511). At each run, the tracker size
is configured to at least double the cache size to satisfy the inequality 
$K \ge 2.C$. 

As shown in Figure~\ref{fig:tracker_size}, the effect of increasing the tracker
size on the cache hit rate follows a repetitive pattern. Initially, increasing 
the tracker size significantly increases the cache hit rate. In fact, for small
cache sizes, doubling tracker size increases the cache hit rate by a factor
of 2.88. Further tracker size doubling enhances cache hit rates by smaller
factors. Afterwards, the cache hit rate stabilizes and increasing the tracker size 
beyond 16 times the cache size  ($K = 16.C$) does not achieve any
additional cache hit rate gains. This experiment suggests to set the tracker size to 
16 times the cache size for this workload. The ideal tracker-to-cache 
size ratio differs from one workload distribution to another. 
In \algoname's adaptive 
resizing algorithm, the tracker-to-cache size ratio is initially configured to 2. The 
first phase of \algoname's resizing algorithm discover the ideal tracker to size ratio
for the current workload. This is achieved by fixing the cache size and doubling
the tracker size until the hit-rate stabilizes. 

\begin{figure}[ht!]
    \includegraphics[width=\columnwidth]{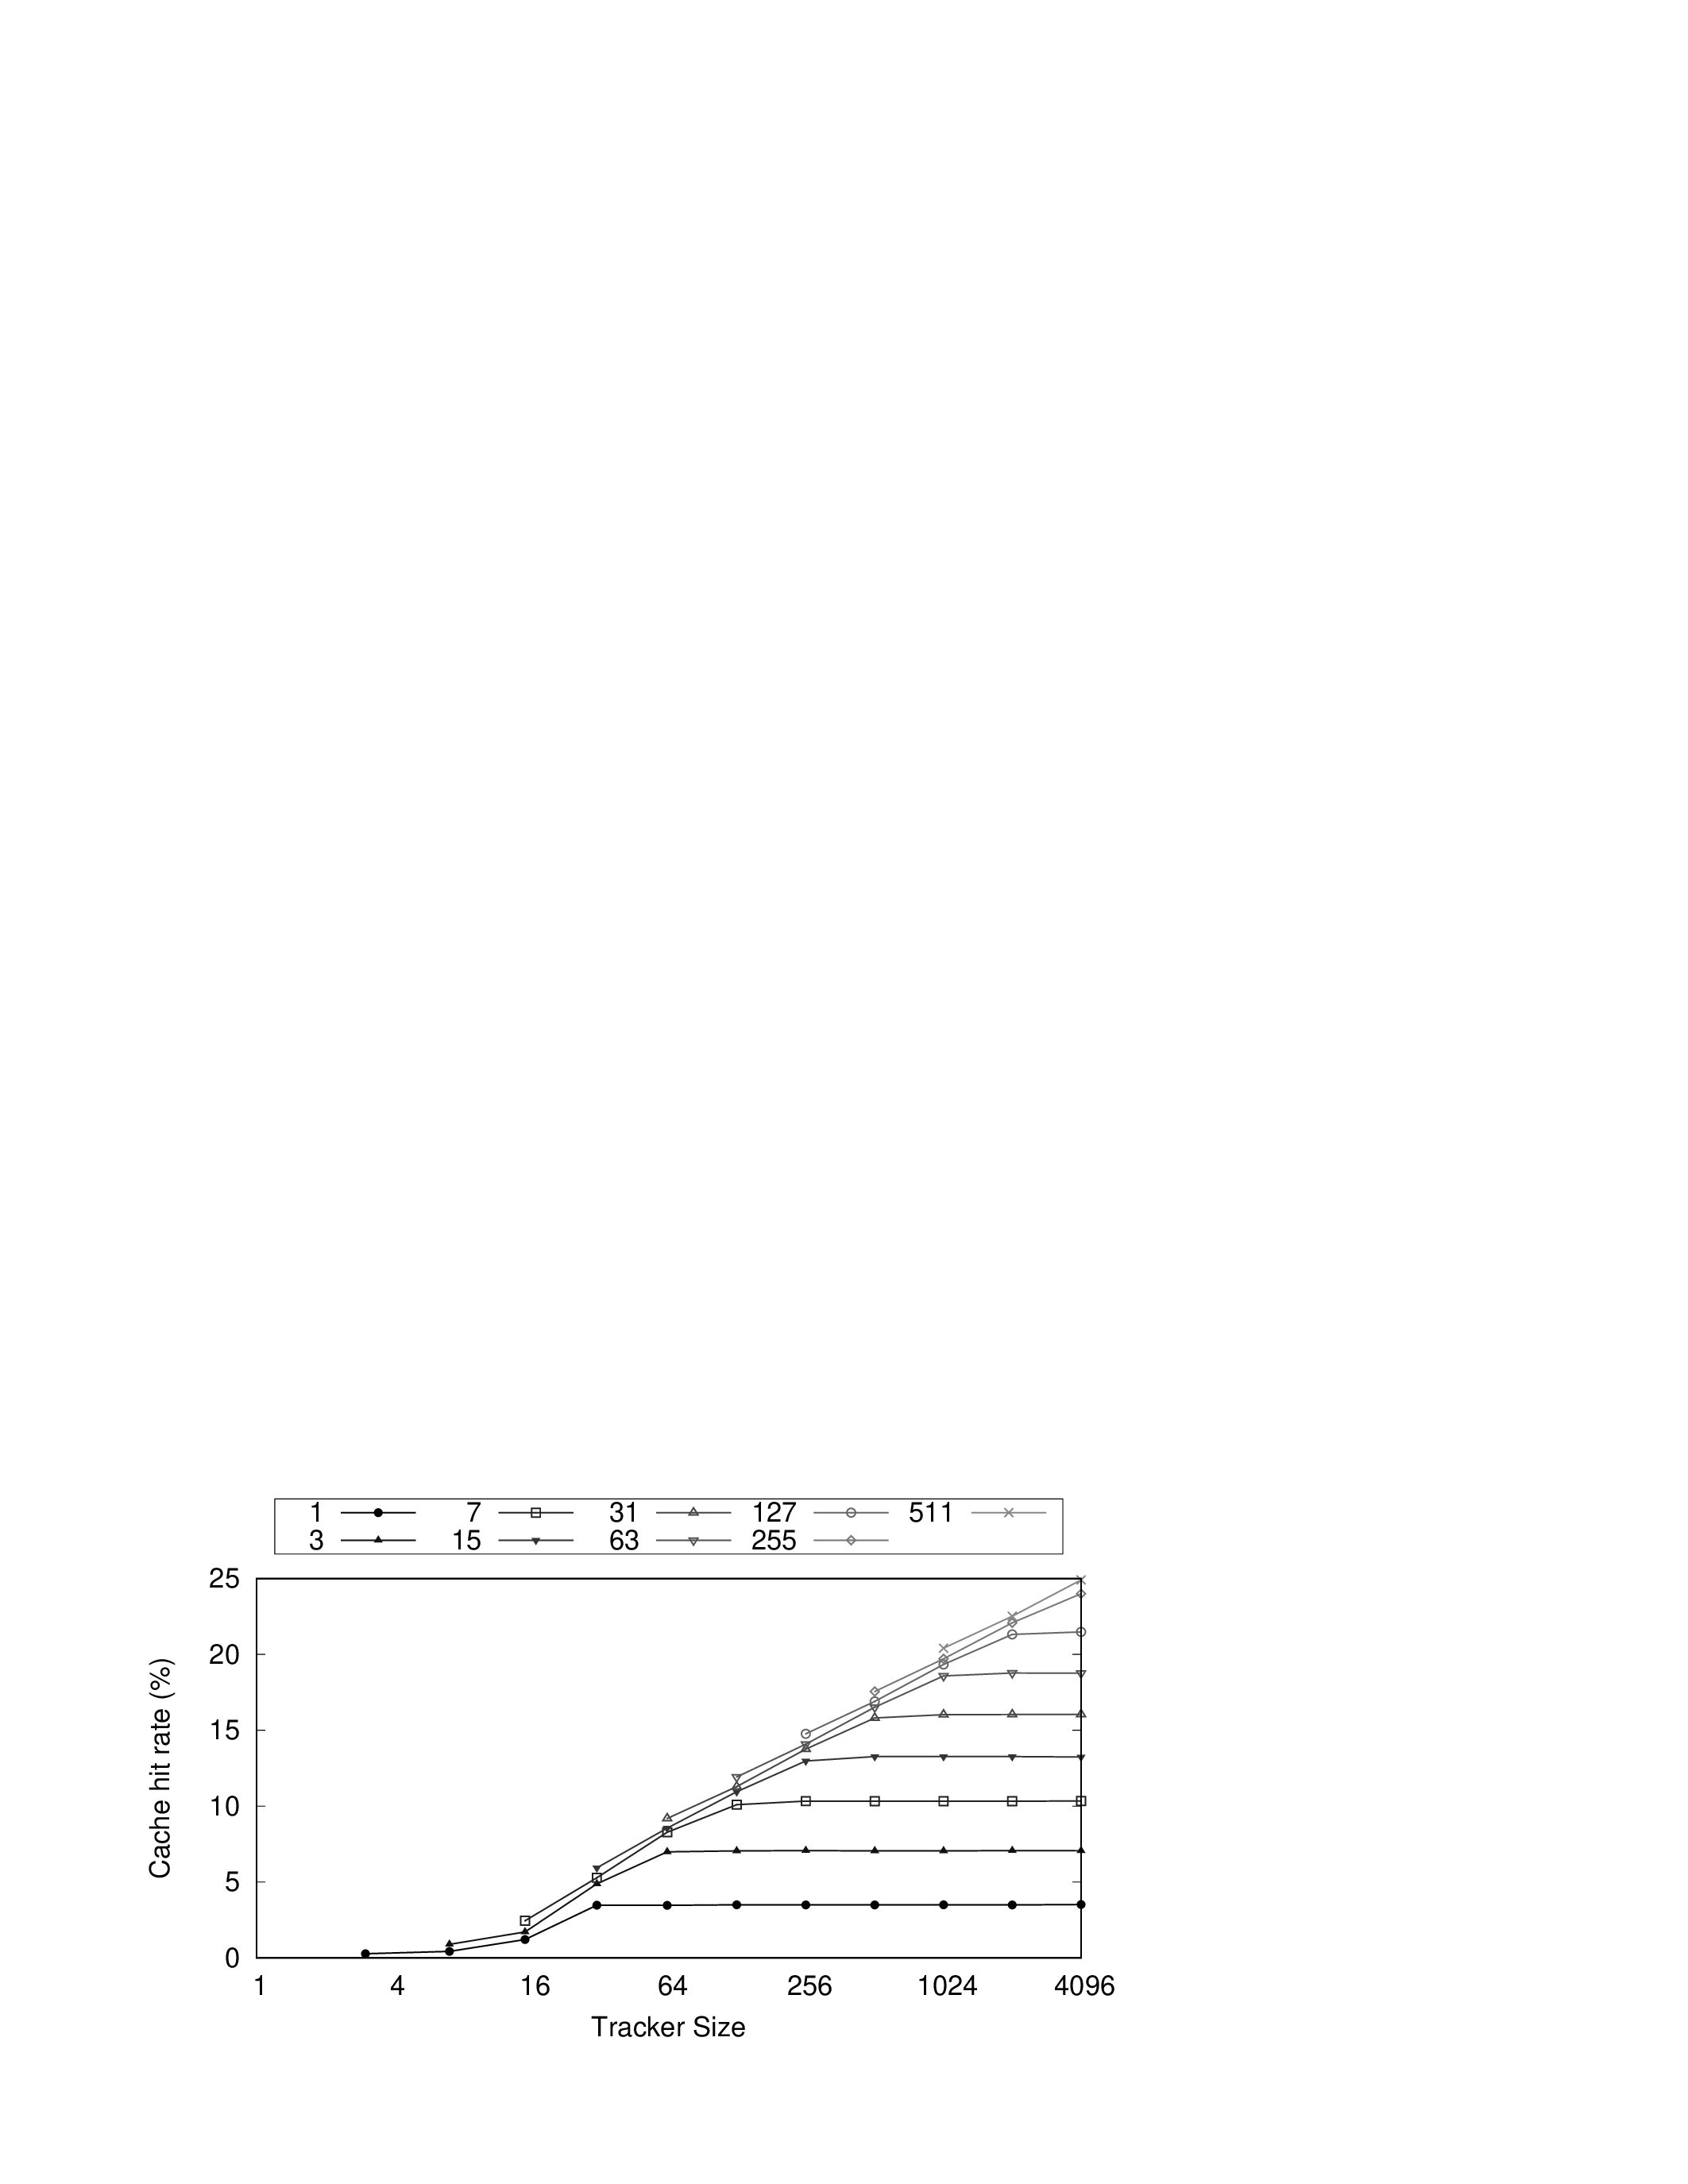}
    \caption{The effect of varying tracker size while fixing cache size 
    on \algoname's hit rate. Different lines represent different cache sizes.}
    \label{fig:tracker_size}
\end{figure}

% System administrators can use \algoname's adaptive resizing algorithm to first 
% discover the ideal cache size

\end{appendices}
